# Supplementary material for: Coopetitive Soft Gating Ensemble
Source: arXiv:1807.01020 source file (2018-08-16)
Supplement: Supplementary file 1 [file appendix.tex]

\appendix
\section{Anhang}
\captionsetup{list=no}

Im Anhang können Sie zusätzliche Bilder der Experimente oder mathematische Beweise anhängen, wenn dies Ihrer Arbeit erfordert.
